# Supplementary material for: Differentially Private Nonparametric Hypothesis Testing
Source: arXiv:1903.09364 source file (2019-03-22)
Supplement: Supplementary file 1 [file KW_Square_type_1.tex]

The question arises: what if the (public) number of groups is "inaccurate:" $\data$ contains empty groups. Are our results still valid if we run the test with too many groups?

Let $g_r$ be the number of groups such that $n_i >0$; it follows that $g_r \leq g$. When we generate the null distribution in the public setting, we need $g_r-1$ for the degrees of freedom in the $\chi^2$ distribution. However, in the differentially private setting, $g_r$ is private information and so it cannot be used to generate the private null distribution. 

But since $g_r \leq g$, for the same $\alpha$, the critical values of $\chi^2(g-1)$ are always larger than those of $\chi^2(g_r-1)$. Thus, $$\Pr[Z>z'^*]<\Pr[Z>z^*]=\Pr[Z'>z'^*]=\alpha,$$ where $Z,\ Z'$ are random variables when $g_r<g$ and $g_r = g$, respectively, and $z^*, \ z'^*$ are critical values for the distributions of $Z$ and $Z'$, respectively.

Therefore, assuming that all $g$ groups have elements and using $g$ to generate the null distribution will make the type I error smaller, and thus our results are valid (but will cause some power loss).
